# Supplementary material for: Robust Accelerated Primal-Dual Methods for Computing Saddle Points
Source: arXiv:2111.12743 source file (2024-09-01)
Supplement: Supplementary file 1 [file ex_supplement.tex]

% SIAM Supplemental File Template
\documentclass[review,supplement,onefignum,onetabnum]{siamart190516}
\usepackage{xr}
% \input{ex_shared}

% The next statement enables references to information in the
% supplement. See the xr-hyperref package for details.
\makeatletter
\newcommand*{\addFileDependency}[1]{% argument=file name and extension
  \typeout{(#1)}
  \@addtofilelist{#1}
  \IfFileExists{#1}{}{\typeout{No file #1.}}
}
\makeatother

\newcommand*{\myexternaldocument}[1]{%
    \externaldocument{#1}%
    \addFileDependency{#1.tex}%
    \addFileDependency{#1.aux}%
}
\myexternaldocument{arXiv_v1}


% Optional PDF information
\ifpdf
\hypersetup{
  pdftitle={Supplementary Materials: ROBUST PRIMAL-DUAL METHODS FOR COMPUTING SADDLE POINTS},
  pdfauthor={X.Zhang，N.S.Aybat, M.Gürbüzbalaban}
}
\fi

\begin{document}

\maketitle



\bibliographystyle{siamplain}
\bibliography{references}
\end{document}
